# Supplementary material for: ARMOR: High-Performance Semi-Structured Pruning via Adaptive Matrix Factorization
Source: arXiv:2510.05528 source file (2026-04-03)
Supplement: Supplementary file 1 [file AdditionalComparisons.tex]

\red{There has been a growing body of work in the community on learnable semi-structured pruning frameworks. Three notable methods are MaskLLM \citep{fang2024maskllm}, RotPrune \citep{chen2025rotpruner}, DenoiseRotator \citep{gu2025denoiserotator}. Here we explicitly position \method vs these works.}

\subsection{Regime Difference (vs. MaskLLM):}
\red{
\method is a strict One-Shot method (no retraining), whereas MaskLLM operates in a Retraining regime, by parameterizing the sparse masks as gumble softmaxes and training them. Comparing \method with MaskLLM is an apples-to-oranges comparison. \textbf{\method uses 4000$\times$ less data} (128 samples vs 512k samples) and \textbf{80$\times$} less compute (16 A6000 GPU hours vs 1280 A100 hours) than MaskLLM.
}

\subsection{Structural Difference (vs. Rotation Methods):} 
\red{RotPruner and DenoiseRotator enhance sparsity by rotating the weight basis using orthogonal matrices. In contrast, \method factorizes the weights using Block-Diagonal wrappers. This block-diagonal structure allows for a directly tunable overhead (via block size) vs the fixed overhead of Rotation methods. Furthermore, unlike RotPruner/DenoiseRotator, which rely on transformer-specific rotation strategies, \method factorizes linear layers agnostically, making it compatible with any architecture using linear projections. Below we compare against RotPrune and DenoiseRotator individually.}\par
\red{
\textbf{RotPrune:} In Table \ref{tab:rotpruner} we compare Wikitext2 perplexities at context length 2048 between \method and RotPrune for Llama-2 7B and Llama 3 8B. \method significantly outperforms RotPruner on both. A full comparison is not possible because there is no public code for RotPrune.}\par
\input{Tabels/Additional Comparisons/RotPruner}
\red{
\textbf{DenoiseRotator:} In Table \ref{tab:denoise} we compare Wikitext2 perplexities at context length 2048 between \method and DenoisePruner on Llama-2 7B/13B/70B and Llama-3 8B. \method outperforms Wanda+DenoisePruner across all models and is competitive with SparseGPT+DenoisePruner.
\input{Tabels/Additional Comparisons/DenoiseRotator}
}
